# Supplementary material for: Influence-Driven Explanations for Bayesian Network Classifiers
Source: arXiv:2012.05773 source file (2021-03-10)
Supplement: Supplementary file 1 [file sm_datasets.tex]

\begin{tabular}{r|cc|cc|cc|cc}
Setting & Data Source$^{*}$  & Classifier Implementation$^{\dagger}$ \\
\hline
\textbf{Shuttle} & DT & \code{skl}\\
\textbf{Parole} & DT & \code{skl}\\
\textbf{German} & DT & \code{skl}\\
\textbf{COMPAS} & DT & \code{skl}\\
\textbf{Car} & DT & \code{skl}\\
\textbf{Emotions} & DT & Chain of \code{skl}\\
\textbf{Asia} & BN & Chain of \code{pgm}\\
\textbf{Child} & BN & Chain of \code{pgm}\\
\end{tabular}
